# Supplementary material for: Lalaine: Measuring and Characterizing Non-Compliance of Apple Privacy Labels at Scale
Source: arXiv:2206.06274 source file (2022-06-19)
Supplement: Supplementary file 1 [file appendix.tex]

\section{Location}

Note that in the new ACM style, the Appendices come before the References.

\begin{table}[ht]
\centering
\footnotesize
\caption{Request}
\begin{tabular}{l|c}
\hline
authorization information (AUI) & access\_token,oauth\_service \\ \hline
personal information (PII) & email, first\_name,last\_name, address, city, postcode, country,gender   \\ \hline
advertising information (ADI) & adurl, adslots, is\_origin\_ad, publisher\_timeout\_control, idfv,  ad\_sdk\_version, accepted\_size, width, height, ad\_count,fbs\_aeid, skadn\_registered\_at\\ \hline
user behavior information (UBI) & log time, xwhen, xwho, xwhat, is\_first\_day, is\_login, first\_visit\_time, first\_visit\_language, is\_from\_background,subscription\_start\_date \\ \hline

\end{tabular}
\label{table:request}
\end{table}

\begin{table}[ht]
\centering
\footnotesize
\caption{Response}
\begin{tabular}{l|c}
\hline
registration data (RED)  & create time \\ \hline
first party advertisement data (FAD) & xxx \\ \hline
measurement data (MD) & xxx \\ \hline
third party advertisement data (TAD) & xxx \\ \hline
marketing metrics (MM) & xxx \\ \hline

\end{tabular}
\label{table:request}
\end{table}

\begin{table*}[ht]

\centering
\footnotesize
\caption{Summary}
\begin{tabular}{c|c|c|c|c|c|c|c|c|c}
\hline
Caller & API  & Frequency  & Endpoint Role$^\ddag$    & Request & Response  & First Level Property& Second Level Purpose &OP$^\dag$\\ \hline

App  & System API   &only once   & ADC& AUI $\wedge$ PII &  RED  & Data linked to the user &App functionality &Y  \\\hline

Third-party  & System API  & Frequently   & TAD  & FADI $\wedge$ PII & TAD   & Data linked to the user &Third-Party Advertising &N \\\hline

Third-party  & System API  & Frequently   & TAN & UBI $\wedge$ PII & MD  & Data linked to the user & Analytics &N \\\hline

App $\vee$ Third-party  & System API  & Frequently   & ADC $\vee$ TAM & TADI $\wedge$ PII & MM $\vee$ FAD  & Data linked to the user & Developer’s Advertising or Marketing &N \\\hline
 \\\hline
 
\end{tabular}
\begin{flushleft}
$\dag$: Optional Disclosure.\\
$\ddag$: Endpoint Role: Third-party Advertiser:TAD,  Third-party analytics: TAN, Third-party measurement or marketing: TAM, App Developer Company: ADC, Third-party app maker: TAM.
%Android 10 additionally requires a \texttt{XXX} permission when XXX in the backgroud.} \haoran{please fill and check.

\end{flushleft}
\label{table:pattern}
\end{table*}

%\begin{acks}
% TODO: For the submission, don't include acknowledgments since they would most likely deanonymize you.
%\end{acks}
